# Supplementary material for: Planning in Markov Decision Processes with Gap-Dependent Sample Complexity
Source: arXiv:2006.05879 source file (2020-06-10)
Supplement: Supplementary file 1 [file worsecase.tex]

\subsection{Sample Complexity scaling with a Near-Optimality Dimension} \label{appendix:worsecase}

In the deterministic case a policy $\pi = \pi_{1:H}$ exactly corresponds to a sequence of states and actions, hence we write $\pi = (s_1,a_1,\dots,s_{H},a_H)$. 

We first rewrite the gap of a partial policy 
\[\Delta^2(\pi_{1:h}) = \frac{(V(\pi_{1:1}) - V(\pi_{1:h}) - \gamma^h \sigma_{H-h})^2_+}{2\sigma_h^2}\]
and that of a complete policy 
\[\Delta^2(\pi_{1:H}) = \max_{h=1}^H \frac{\tilde{\Delta}_h^2(s_h,a_h)}{8\sigma_{H-h+1}^2} \vee \max_{h=2}^H \frac{(V(\pi_{1:1}) - V(\pi_{1:h}) - \gamma^h \sigma_{H-h})^2_+}{2\sigma_{h}^2}\]
%It can be shown that $V(\pi_{1:1}) - V(\pi_{1:h}) = \sum_{\ell=2}^h \gamma^{\ell-1} \Delta_{\ell}(s_{\ell},a_{\ell})$. 
As $\tilde\Delta_1^\star(s_1,a_1) \geq \Delta \vee \epsilon$, all the policies satisfy in particular $\Delta^2(\pi_{1:H}) \geq \frac{\Delta^2\vee \epsilon^2}{8\sigma_{H}^2}$.

In the discounted setting, the planning horizon $H$ is chosen such that $\frac{\gamma^H}{1-\gamma} \simeq \epsilon$ to guarantee an approximation error is of order $\epsilon$. In that case, Corollary~\ref{cor:generalSC} yields that with high probability
\[\tau_\delta = O \left(\frac{K^H}{\Delta^2\vee \epsilon^2}\right) = O\left(\frac{1}{\Delta^2\vee \epsilon^2} \left(\frac{1}{\epsilon}\right)^{\frac{\ln(K)}{\ln(1/\gamma)}}\right).\]

The factor $K$ can be replaced by some notion of \emph{near-optimality dimension}, by considering a well-chosen admissible partition, in the sense of Definition~\ref{def:partition}. 

For $h\geq 2$, we define the set of near-optimal partial policies of length $h$ as 
\[\cI_h = \left\{V(\pi_{1:1}) - V(\pi_{1:h}) \leq \frac{2\gamma^{h}}{1-\gamma} \right\}\]
If $\pi_{1:h} \notin \cI_h$, observe that $\Delta^2(\pi_{1:h}) \geq \frac{\gamma^{2h}}{2(1 - \gamma^h)^2}$. 
Letting \[\cJ_h = \left\{\pi_{1:h} : \pi_{1:h} \notin \cI_h \text{ and } \pi_{1:(h-1)} \in \cI_{h-1} \right\},\]
there exists an admissible partition $\cP=\{(\pi^1,h^1),\dots,(\pi^L,h^L)\}$ such that either $h^i = H$ and $\pi^i_{1:H} \in \cI_H$ or $\pi^i_{1:h_i} \in \cJ_{h_i}$, which implies $\Delta^2(\pi^i_{1:{h^i}}) \geq \frac{\gamma^{2{h^i}}}{2(1 - \gamma^{h^i})^2}$

% hence on the event $\cE$ we get that 
% \[n^\tau(a_{1:h}) \leq 2 \left(\frac{\sum_{\ell=0}^{h-1}\gamma^\ell}{\sum_{\ell = 0}^{H-h-1}\gamma^\ell}\right)^2 \beta(n^\tau(a_{1:h}) , \delta),\] hence $n^\tau(a_{1:h})= O\left( \left(\frac{\sum_{\ell=0}^{h-1}\gamma^\ell}{\sum_{\ell = 0}^{H-h-1}\gamma^\ell}\right)^2 \ln \left(\frac{(BK)^H}{\delta}\right)\right)$ by Lemma~\ref{lemma:technical}.

On the event $\cE$, 
\begin{eqnarray*}
\tau_\delta &=& \sum_{\substack{i=1\\ h^i = H}}^L n^{\tau}(\pi^i) +   \sum_{\substack{i=1\\ h^i < H}}^L n^{\tau}(\pi^i) \\
& = & O\left(\left[\sum_{\substack{i=1\\ h^i = H}}^L \frac{1}{\Delta^2 \vee \epsilon^2} +   \sum_{\substack{i=1\\ h^i < H}}^L\frac{(1 - \gamma^{h^i})^2}{\gamma^{2{h^i}}}\right]\ln\left(\frac{(BK)^H}{\delta}\right)\right) \\
& \leq & O\left(\left[|\cI_H| \frac{1}{\Delta^2 \vee \epsilon^2} +   \sum_{h=3}^{H} |\cJ_h|\frac{(1 - \gamma^{h})^2}{\gamma^{2{h}}}\right]\ln\left(\frac{(BK)^H}{\delta}\right)\right)\\
& \leq & O\left(\left[|\cI_H| \frac{1}{\Delta^2 \vee \epsilon^2} +   \sum_{h=3}^{H} K|\cI_{h-1}|\gamma^{-2h}\right]\ln\left(\frac{(BK)^H}{\delta}\right)\right)
\end{eqnarray*}
Defining the near optimality dimension to be such that $|\cI_h| \simeq \kappa^h$ yields that on $\cE$
\[\tau_\delta = O\left(\left[\frac{\kappa^H}{\Delta^2\vee \epsilon^2}+ \left(\kappa\gamma^{-2}\right)^H\right]\ln\left(\frac{(BK)^H}{\delta}\right)\right).\]
Selecting $H \simeq \ln(1/\epsilon)/\ln(1/\gamma)$ one obtains $\kappa^H \simeq \left(\frac{1}{\epsilon}\right)^{\frac{\ln(\kappa)}{\ln(1/\gamma)}}$ and $\left(\kappa\gamma^{-2}\right)^H \simeq \left(\frac{1}{\epsilon}\right)^{\frac{\ln(\kappa)}{\ln(1/\gamma)}+2}$, hence $\tau_\delta  = \tilde{O}\left(\epsilon^{-\left[\frac{\ln(\kappa)}{\ln(1/\gamma)}+2\right]}\right)$ (ommiting log factors).
